# Supplementary material for: Electronic structure quantum Monte Carlo
Source: arXiv:1008.2369 source file (2010-08-13)
Supplement: Supplementary file 1 [file caylesproof.tex]

\subsection{Proof of Cayley's Identity}\label{appendix:Cayley}
In order to prove the statement in Eq.~(\ref{eq:cayley}) we will proceed by induction. For $n=2$ it is true that
\begin{equation*}
{\rm det} \left[\begin{array}{cc}
0  & b_{12} \\
-a_{12}  & 0 \end{array}\right]
={\rm pf} \left[\begin{array}{cc}
0  & b_{12}\\
-b_{12} & 0\end{array}\right]
{\rm pf} \left[\begin{array}{cc}
0  & a_{12} \\
-a_{12} & 0\end{array}\right].
\end{equation*}
For even $n$ greater than $2$, determinant of our matrix of interest 
can be expanded through its cofactors as
\begin{align}\label{eq:a:expand}
 {\rm det}& \left[\begin{array}{ccccc}
0  & b_{12}  & b_{13} &\ldots &  b_{1,n}\\
-a_{12}  & 0  & a_{23} & \ldots &  a_{2,n}\\
-a_{13}  & -a_{23} & 0  & \ldots &  a_{3,n}\\
 \vdots & \vdots & \vdots &  \ddots &  \vdots \\
-a_{1,n} & -a_{2,n} & -a_{3,n} & \ldots &  0\\
\end{array}\right]=\sum_k -a_{1,k} C(k,1) \nonumber \\ 
&=\sum_k  \sum_l  -a_{1,k} b_{1,l} C(k,1;1,l)
\end{align}
%Here we note that the double cofactor of our matrix for $k$-th row and $l$-th
%column does not contain any of the first row/column elements.
The cofactor can be written as
%\begin{widetext}
%\small
\begin{equation}
C(k,1;1,l)=(-1)^{k+l+1}{\rm det} \left[A(k,1;1,l)\right],
\end{equation}
where the cofactor matrix  is given by
\begin{equation}
\small
A(k,1;1,l)=
\left[
\begin{array}{ccccccc}
0 & a_{23}  & \ldots & a_{2,k} & \ldots &  a_{2,n}\\
-a_{23}  & 0  & \ldots &  a_{3,k} & \ldots & a_{3,n}\\
 \vdots & \vdots & \ddots & \vdots & \ddots & \vdots  \\
-a_{2,l} & -a_{3,l} & \ldots & -a_{k,l} &\ldots & a_{l,n}\\
\vdots & \vdots & \ddots & \vdots & \ddots & \vdots  \\
-a_{2,n} & -a_{3,n} & \ldots & -a_{k,n} &\ldots & 0
\end{array}\right].
\end{equation}
At this point we would like to use the induction step and rewrite
the determinant cofactor as a product of two pfaffians [Cayley's identity Eq.~(\ref{eq:cayley})].
This would allow us to demonstrate that the expansion is identical to 
the expansion of pfaffians in minors.
In order to do so, however, we have
to shift the $k$-th column by pair column exchanges, so it becomes
the {\em last} column and, similarly, we have to shift the $l$-th row by
pair exchanges, so it becomes the last row.
This involves $k$ pair exchanges of columns and $l$ pair exchanges or rows and 
can be represented by unitary matrices $U_k$ and $U_l$.
It is necessary to invoke these operations so that the 
matrix gets into a form directly amenable for the Cayley's identity, i.e.,
the matrix has to be in a manifestly skew-symmetric form. 
(The sign change from the row/columns exchanges will prove irrelevant as we will 
show below.)
The transformed matrix is given by 
\begin{equation}
A'(k,1;1,l)=U_kA(k,1;1,l)U_l
\end{equation}
and has all zeros on the diagonal with the exception of the last element which is equal to $-a_{k,l}$. 
The last row is given by
\begin{align} 
{\bf v}_r=&(-a_{2,l},\ldots, -a_{k-1,l},-a_{k+1,l},\ldots \nonumber \\
&\ldots,-a_{l-1,l},a_{l,l+1},\ldots, a_{l,n},-a_{k,l}), 
\end{align}
while the last column is given as following
\begin{align}
{\bf v}_c^T=&(a_{2,k},\ldots,a_{k-1,k},-a_{k,k+1},\ldots \nonumber \\
&\ldots,-a_{k,l-1},-a_{k,l+1},\ldots,-a_{k,n},-a_{k,l})^T.
\end{align}
The only non-zero diagonal element $-a_{k,l}$ can be eliminated, 
once we realize that its cofactor contains a determinant of
a skew-symmetric matrix of odd degree,
which always vanishes (proof by Jacob~\cite{Jacobi}).

Now we are ready to perform the induction step, namely to use the 
property that the determinant of a $2(n-1)\times 2(n-1)$ matrix
can be written as given by the Cayley's identity, Eq.~(\ref{eq:cayley}).
We obtain
\begin{align}
{\rm det}[U_kA(k,1;1,l)U_l]&={\rm det}[A'(k,1;1,l)] \\
 &={\rm pf}[A'(1,k;1,k)]\,{\rm pf}[A'(1,l;1,l)]. \nonumber 
\end{align}
We can now apply the inverse unitary transformations and
shift back the columns (and by the skew-symmetry the corresponding rows) in the
first pfaffian and, similarly, the rows (and corresponding columns) 
in the second. This enables us to write
\begin{align}
{\rm pf}&[A'(1,k;1,k)]\,{\rm pf}[A'(1,l;1,l)]\nonumber \\
&={\rm pf}[U_l^{-1}A(1,k;1,k)U_l]\,{\rm pf}[U_kA(1,l;1,l)U_k^{-1}]\nonumber \\
&={\rm pf}[A(1,k;1,k)]\,{\rm pf}[A(1,l;1,l)],
\end{align}
where we have used the identity given by Eq.~(\ref{eq:pfident4}).
We can therefore finally write
\begin{align}
C(k,1;1,l)&=(-1)^{k+l+1}{\rm pf}[A(1,k;1,k)]{\rm pf}[A(1,l;1,l)] \nonumber \\
&=-P_c(a_{1,k})P_c(a_{1,l}),
\end{align}
where $P_c$ denotes a pfaffian cofactor as defined in (\ref{eq:pfcof}). 
Therefore, the determinant expansion in Eq.~(\ref{eq:a:expand}) equals to
\begin{align}
\sum_{k,l} -a_{1,k} b_{1,l} C(k,1;1,l)&=\sum_{k,l} a_{1,k} b_{1,l} P_c(a_{1,k})P_c(a_{1,l}) \nonumber \\
&={\rm pf}[A]{\rm pf}[B]
\end{align}
with matrices $A$ and $B$ defined as in Eq.~(\ref{eg:inverseupdate}).
This concludes the proof of the more general form of the Cayley's identity. Note, if $B=A$,
we trivially obtain well-known formula for the square of
pfaffian [Eq.~(\ref{eq:pfident2})].
