# Supplementary material for: Electronic structure quantum Monte Carlo
Source: arXiv:1008.2369 source file (2010-08-13)
Supplement: Supplementary file 2 [file Pfaffian_routines.tex]

\subsection{Core Pfaffian Algorithms}\label{appendix:pfaffianroutines}
\subsubsection{Gaussian Elimination with Row-Pivotting Algorithm for Pfaffian Value}
\begin{verbatim}
int RowPivoting(Array2 <doublevar> & tmp, int i, int n){
  //row pivoting algorithm used by Pfaffian_partialpivot
  doublevar big;
  doublevar temp;
  doublevar TINY=1e-20;
  Array1 <doublevar> backup(2*n) ;
  int d=1;
  int k=0;
  big=0.0;
  //find the largest value
  for (int j=i+1;j<2*n;j++){
    temp=fabs(tmp(i,j));
    if(temp > big){
      big=temp;
      k=j;
    }
  }
  if (big<TINY){
    cout <<"Singular row in matrix!!! "<<endl;
    tmp(i,i+1)=TINY;
  }

  if (k!=i+1){
    //exchange k-th column with 2-nd column;
     for (int j=i;j<2*n;j++){
       backup(j)=tmp(j,i+1);
       tmp(j,i+1)=tmp(j,k);
       tmp(j,k)=backup(j);
     }
     //exchange k-th row with 2-nd row;
     for (int j=i;j<2*n;j++){
       backup(j)=tmp(i+1,j);
       tmp(i+1,j)=tmp(k,j);
       tmp(k,j)=backup(j);
     }
     
     d*=-1; //sign change of pfaffian
  }
  return d;
}

doublevar Pfaffian_partialpivot(const Array2 <doublevar> & IN){
  //  returns the pfaffian of skew-symmetric matrix  IN
  //  with partial pivoting
  if (IN.dim[0]%2!=0) return 0.0;
  int n=IN.dim[0]/2;
  Array2 <doublevar> tmp(2*n,2*n);
  doublevar PF=1.0;
  doublevar fac;
  for (int i=0;i<2*n;i++)
    for (int l=0;l<2*n;l++)
      tmp(i,l)=IN(i,l);
 
  int d=1;
  for (int i=0;i<2*n;i=i+2){
    //for given row look for pivoting element
    //exchange if needed
    d*=RowPivoting(tmp, i, n);

    for (int j=i+2;j<2*n;j++){
      fac=-tmp(i,j)/tmp(i,i+1);
      for (int k=i+1;k<2*n;k++){
        tmp(k,j)=tmp(k,j)+fac*tmp(k,i+1);
        tmp(j,k)=tmp(j,k)+fac*tmp(i+1,k);
      }
    }
    PF=PF*tmp(i,i+1);
  }
  return PF*d;
}
\end{verbatim}

\subsubsection{Algoritm for the Update of Inverse of Pfaffian Matrix}
\begin{verbatim}
doublevar UpdateInversePfaffianMatrix(Array2 <doublevar> & IN, 
                                      Array1 <doublevar> & row, 
                                      Array1 <doublevar> & column, 
                                      int e)
{
  //update row and column of skew-symmetric inverse matrix IN
  //the ratio of new/old pfaffians is returned by Column(e)
  int n=in.dim[0]/2;
  for (int i=0;i<2*n;i++){
    column(i)=0.0;
    for (int j=0;j<2*n;j++)
      column(i)+=row(j)*IN(j,i);
  }
  
  //to avoid the catastrophe in later division
  if (column(e)==0)
    column(e)=1e-20;

  //rest is just the new inverse matrix IN
  for(int i=0;i<2*n;i++){
    if (i==e){
      IN(i,i)=0.0;
    }
    else {
      IN(e,i)=+IN(e,i)/column(e);
      IN(i,e)=-IN(e,i);
    }
  }

  for(int j=0;j<2*n;j++){
    if (j!=e){
      for (int k=0;k<2*n;k++){
        if (k==j) {
          IN(k,k)=0.0;
        }
        else {
          IN(k,j)-=column(j)*IN(k,e);
          IN(j,k)=-IN(k,j);
        }
      }
    }
  }
  //return the ratio of pfaffians
  return  column(e);
}
\end{verbatim}
