# Supplementary material for: Electronic structure quantum Monte Carlo
Source: arXiv:1008.2369 source file (2010-08-13)
Supplement: Supplementary file 3 [file Backflow_appendix.tex]

\chapter{Value, Gradient and Laplacian of Back-Flow Wave Function}
