# Supplementary material for: Electronic structure quantum Monte Carlo
Source: arXiv:1008.2369 source file (2010-08-13)
Supplement: Supplementary file 4 [file besselfunctionsandmore.tex]

\subsection{Cutoff-Cusp and Polynomial Pad\'e Functions}\label{appendix:functions}
The exact electron-electron cusp conditions are satisfied by the choice of following cusp-function [see Fig.~(\ref{fig:cutofffunc})]
with variable $x=r/r_{cut}$,  where $r_{cut}$ is some cutoff radius and $\gamma$ is the curvature as  
\begin{align}\label{eq:appendix:functions:1}
f_{cusp}(x,\gamma)=C\left(\frac{x-x^2+x^3/3}{1+\gamma(x-x^2+x^3/3)}-\frac{1}{\gamma+3}\right)
\end{align}
The cusp constant is $C=\frac{1}{4}$ for electrons with like and $C=\frac{1}{2}$ for electrons with unlike spins.  
\begin{figure}[!t]
\begin{center}
\includegraphics[width=0.8\columnwidth]{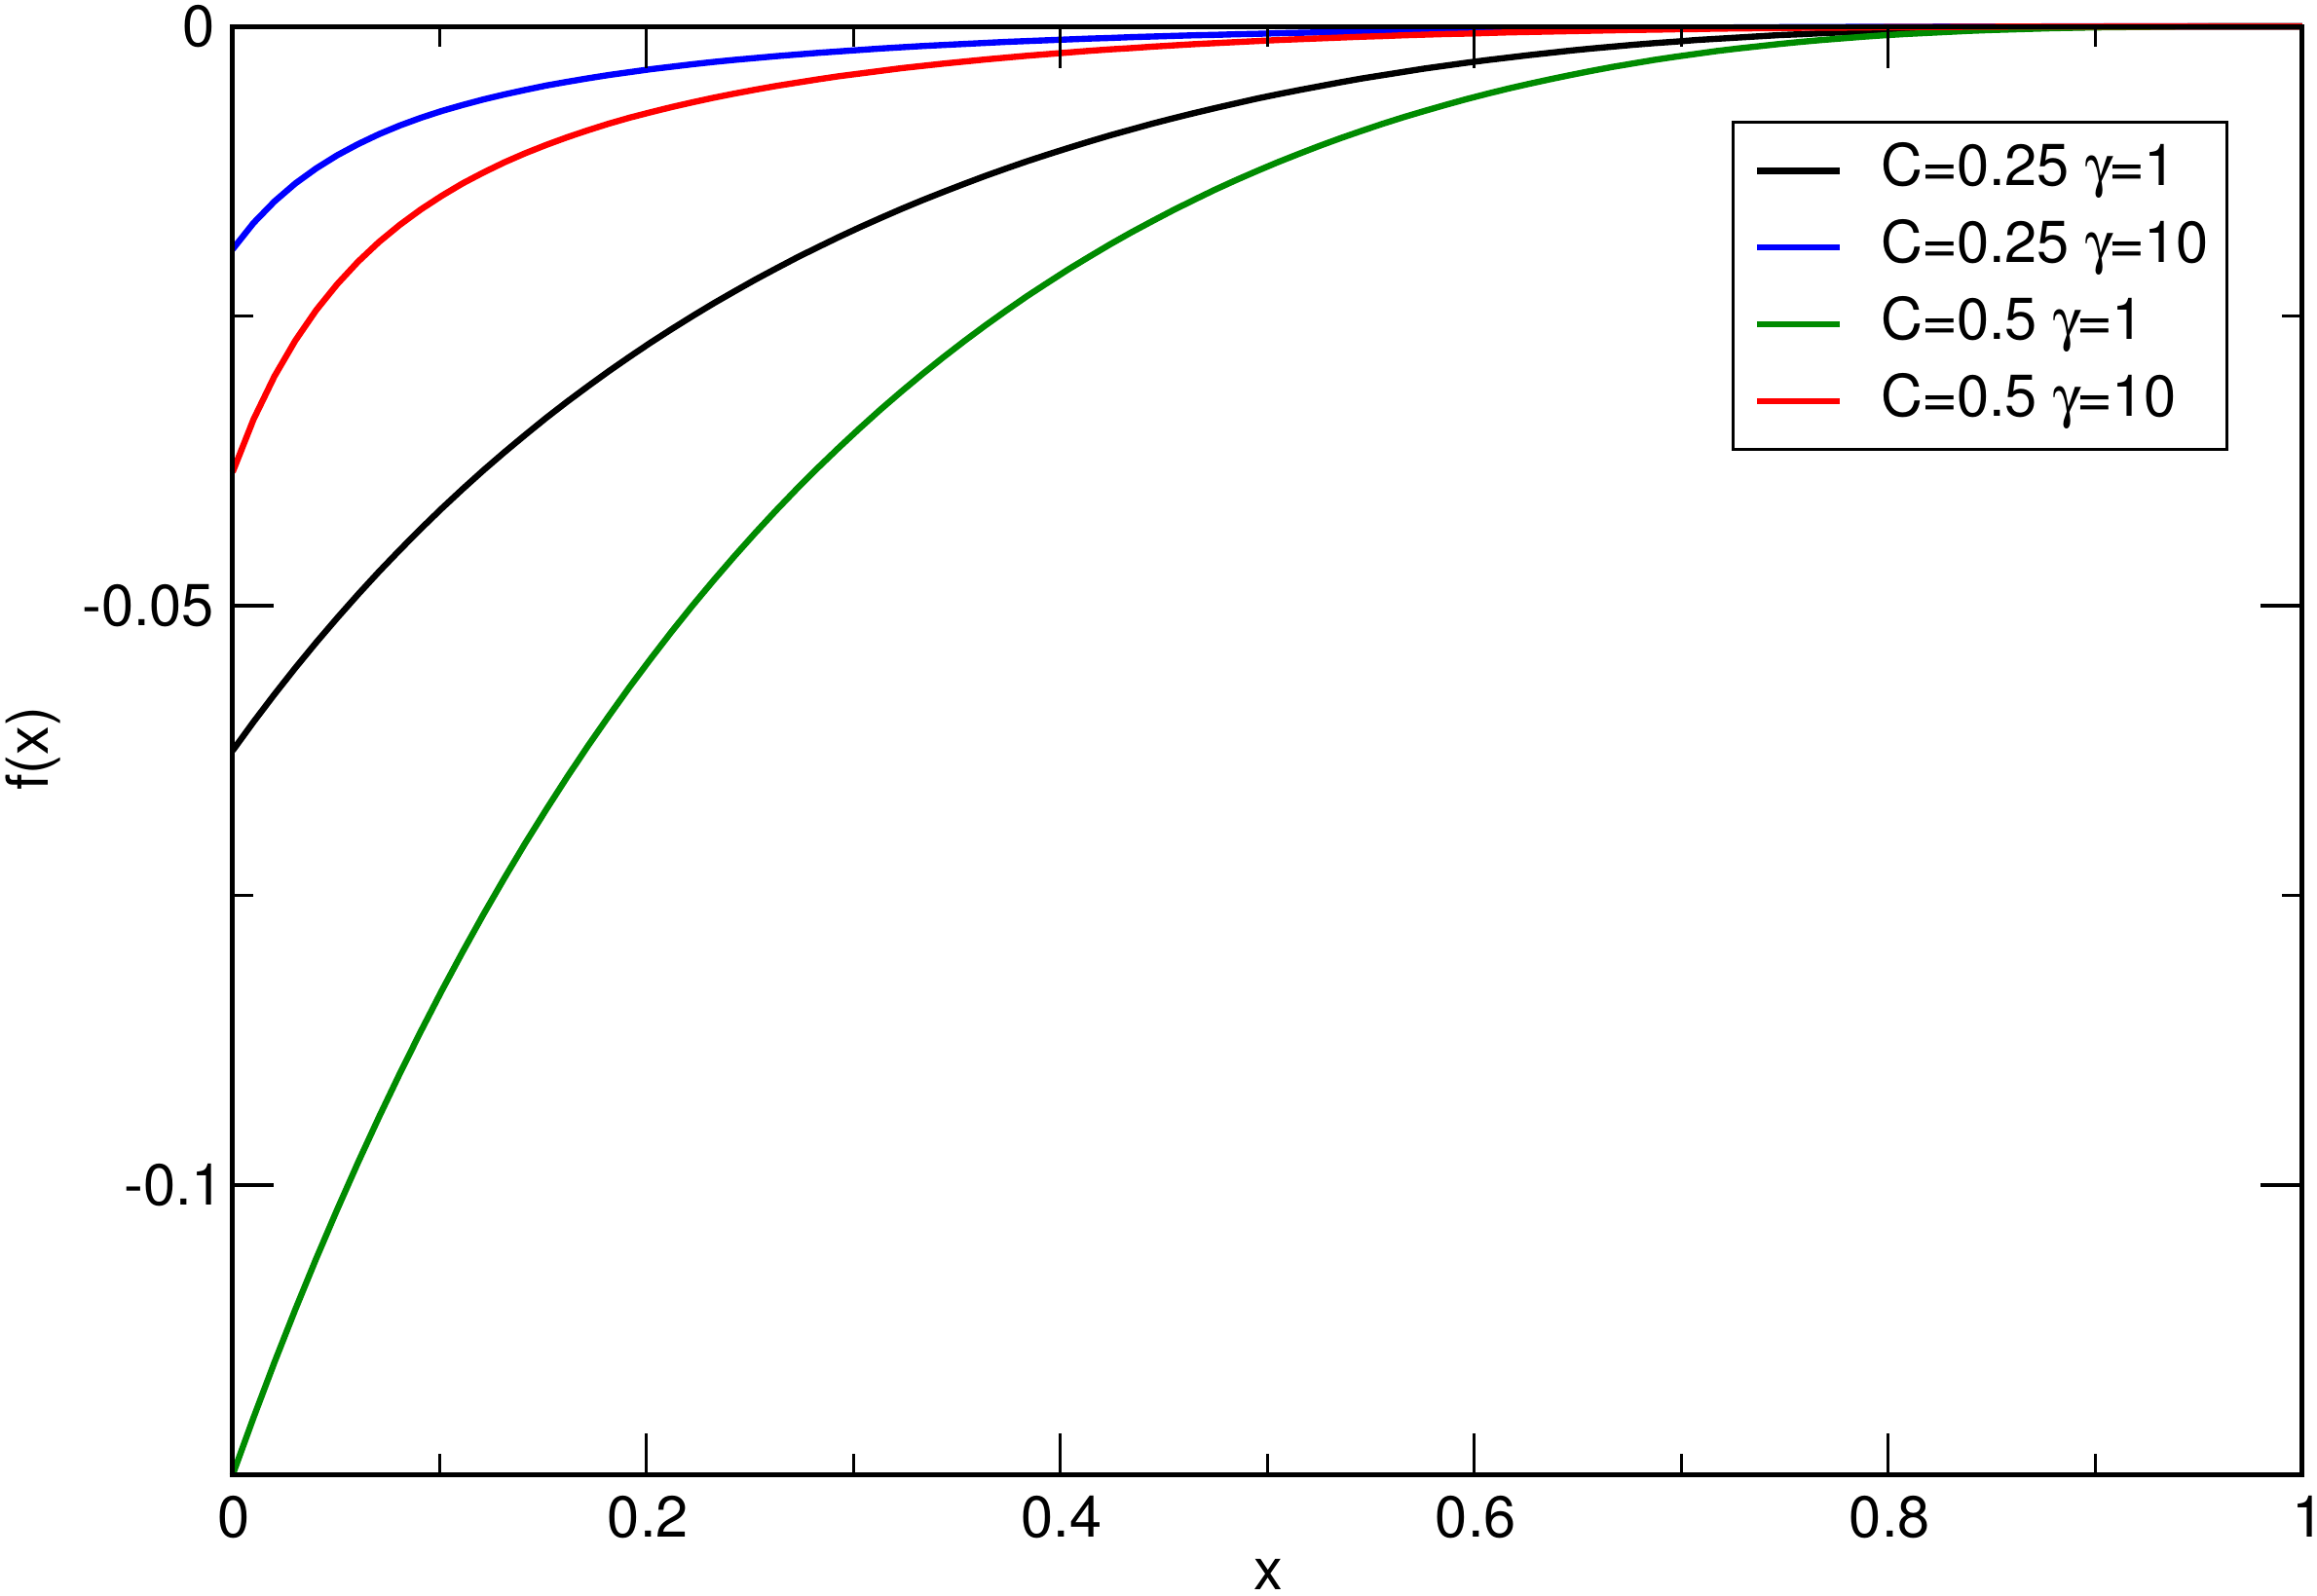}
\end{center}
\caption{Cutoff-Cusp functions with two different curvatures ($\gamma=1$ and $\gamma=10$) for like ($C=\frac{1}{4}$) and 
unlike ($C=\frac{1}{2}$) spins.}
\label{fig:cutofffunc}
\end{figure}

Polynomial Pad\'e functions for the same variable $x=r/r_{cut}$ and curvature $\beta$ had proved to 
be excellent choice for describing the electron-electron and electron-nucleus correlation. In calculations, we use 
the form 
\begin{align}
f_{poly-Pade}(x,\beta)=\frac{1-x^2(6-8x+3x^2)}{1+\beta x^2(6-8x+3x^2)}
\end{align}
The $f_{poly-Pade}(0)=1$ with derivative $f'_{poly-Pade}(0)=0$ and also goes smoothly to zero as $r \to r_{cut}$ [see Fig.~(\ref{fig:bessel})].
These conditions are necessary for preserving cusp conditions already fixed by cusp-functions~(\ref{eq:appendix:functions:1}) and choice of orbitals or pseudopotentials. 
\begin{figure}[!b]
\begin{center}
\includegraphics[width=0.8\columnwidth]{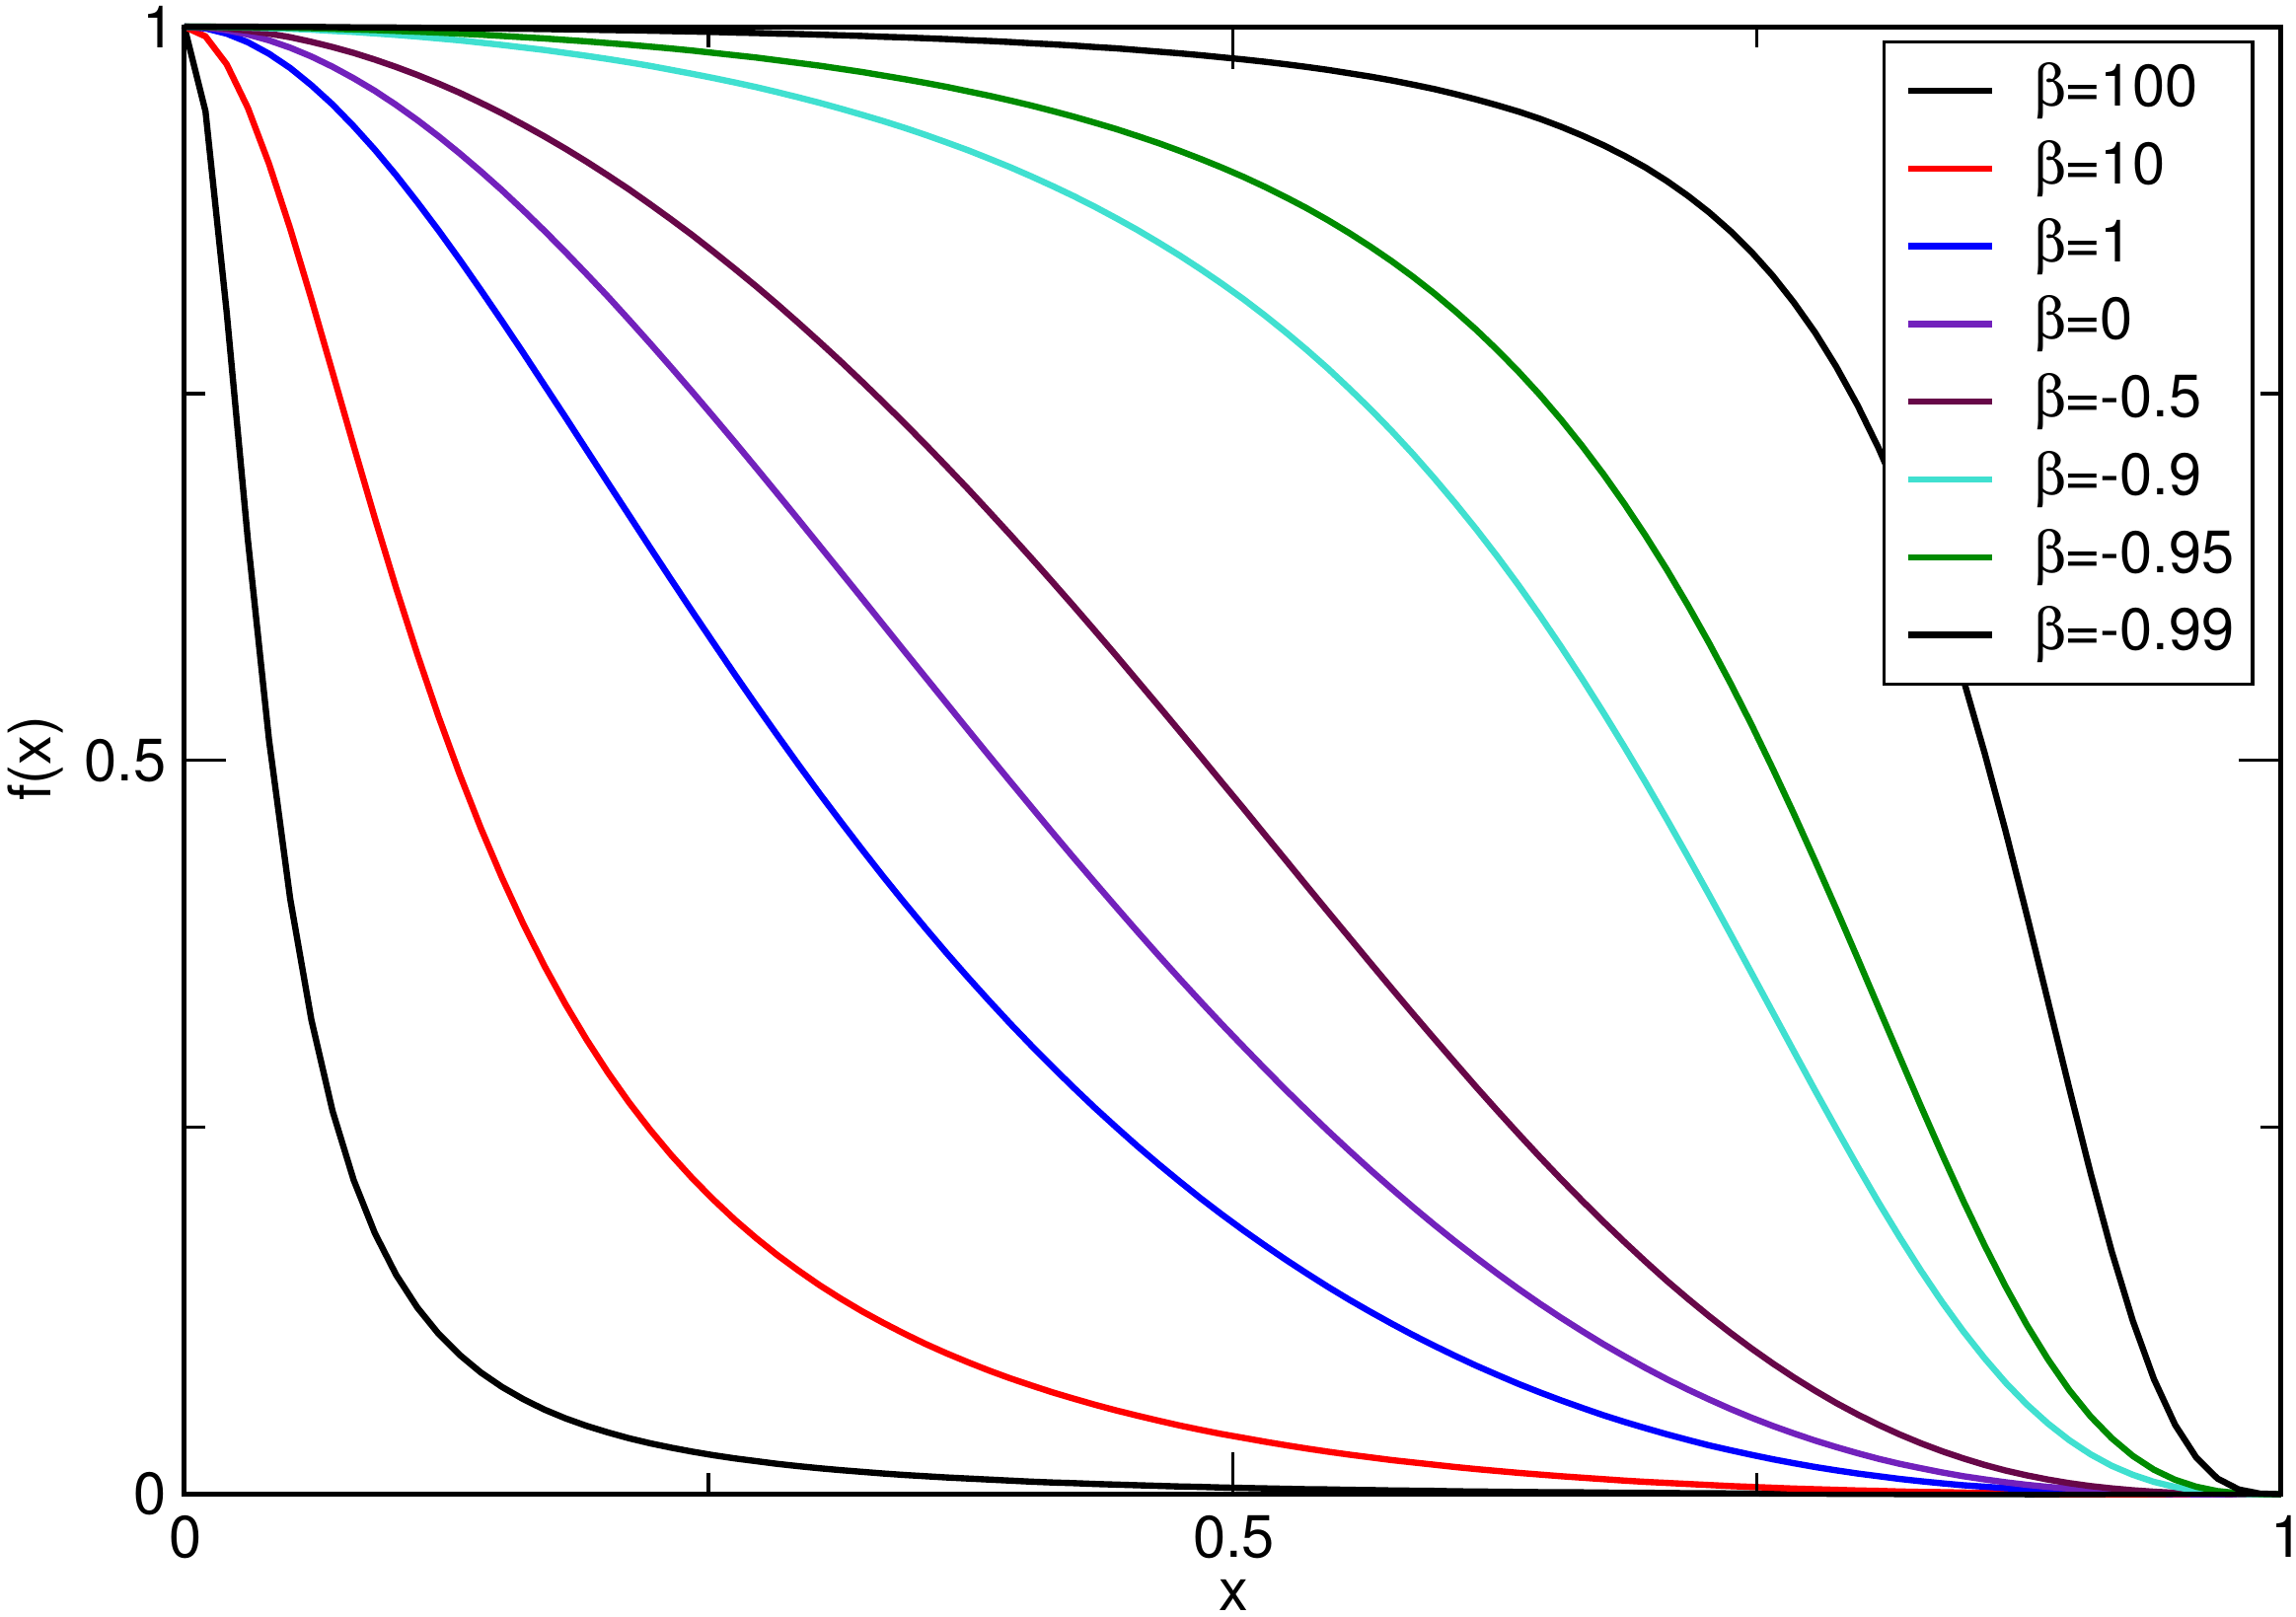}
\end{center}
\caption{Polynomial Pad\'e functions with curvatures $\beta$ ranging from -0.99 to 100.}
\label{fig:bessel}
\end{figure}
