# Supplementary material for: Electronic structure quantum Monte Carlo
Source: arXiv:1008.2369 source file (2010-08-13)
Supplement: Supplementary file 5 [file determinant_analytic_ders.tex]

\chapter{Analytic Derivatives of Determinantal Wave Function  
with Respect to Variational Parameters}
