# Supplementary material for: Electronic structure quantum Monte Carlo
Source: arXiv:1008.2369 source file (2010-08-13)
Supplement: Supplementary file 6 [file pfaffian_analytic_ders.tex]

\chapter{Analytic Derivatives of Pfaffian Pairing Wave Function 
with Respect to Variational Parameters}\label{appendix:pfaffianders}
